# Supplementary material for: SynthForge: Synthesizing High-Quality Face Dataset with Controllable 3D Generative Models
Source: arXiv:2406.07840 source file (2024-06-12)
Supplement: Supplementary file 1 [file X_suppl.tex]

\clearpage
\setcounter{page}{1}
\maketitlesupplementary

To supplement the main manuscript, in this document, we present the details about the data generation and alignment module used to generate data with multimodal annotations in Sec \ref{sec:alignment}.
In Sec \ref{sec:more_results}, we show extensive qualitative results, comparing our method with existing approaches for datasets concering different facial modalities.

\section{Data Generation \& Alignment Module}
\label{sec:alignment}
As illustrated in Fig. 2(A) in the main paper, we utilise Next3D \cite{next3d} as the method for the 3D-aware generative model in our approach. However, we highlight that a similar approach which leverages 3DMM for fine-tuned control over generation of face images is a suitable substitution for the Next3D pipeline, such as the work presented in OmniAvatar \cite{xu2023omniavatar}.

\paragraph{Sampling Next3D parameters}: The parameters for the FLAME mesh creation are sampled randomly in the range $(-2, 2)$ for shape, expression and pose parameters and denoted as $\beta$, $\psi$, and $\theta$, respectively. For the camera parameters, we sample the field-of-view in the range of $12^{\circ}$ to $27^{\circ}$ (degrees) and create a normalized intrinsic matrix $K_{3\times3}$. We then sample the camera pose with distance from the subject placed at origin as 2.7 meters, and azimuth and elevation each sampled from standard normal distribution and scaled to angles of $(\frac{-\pi}{4}, \frac{\pi}{4})$ and convert to the extrinsic matrix denoted by $[R|t]$. Any 3D point in the world space can be projected to the camera co-ordinate system and then to the image coordinate space, using the projection matrix $P = K \cdot [R | t]$.

\paragraph{FLAME Mesh:} Based on the FLAME parameters, we get the vertices ($v$) and the faces ($f_v$) along with landmarks ($l$) from FLAME \cite{flame}. Furthermore, based on the UV mapping available for FLAME, we prepare a segmentation map in the UV space for the FLAME head mesh (shown in in fig. \ref{fig:flame_uv}) and map the textures to the 3D mesh (shown in fig. \ref{fig:flame_tex}).

\begin{figure}[h]
    \centering
    \begin{subfigure}{0.45\columnwidth}
        \includegraphics[width=\columnwidth]{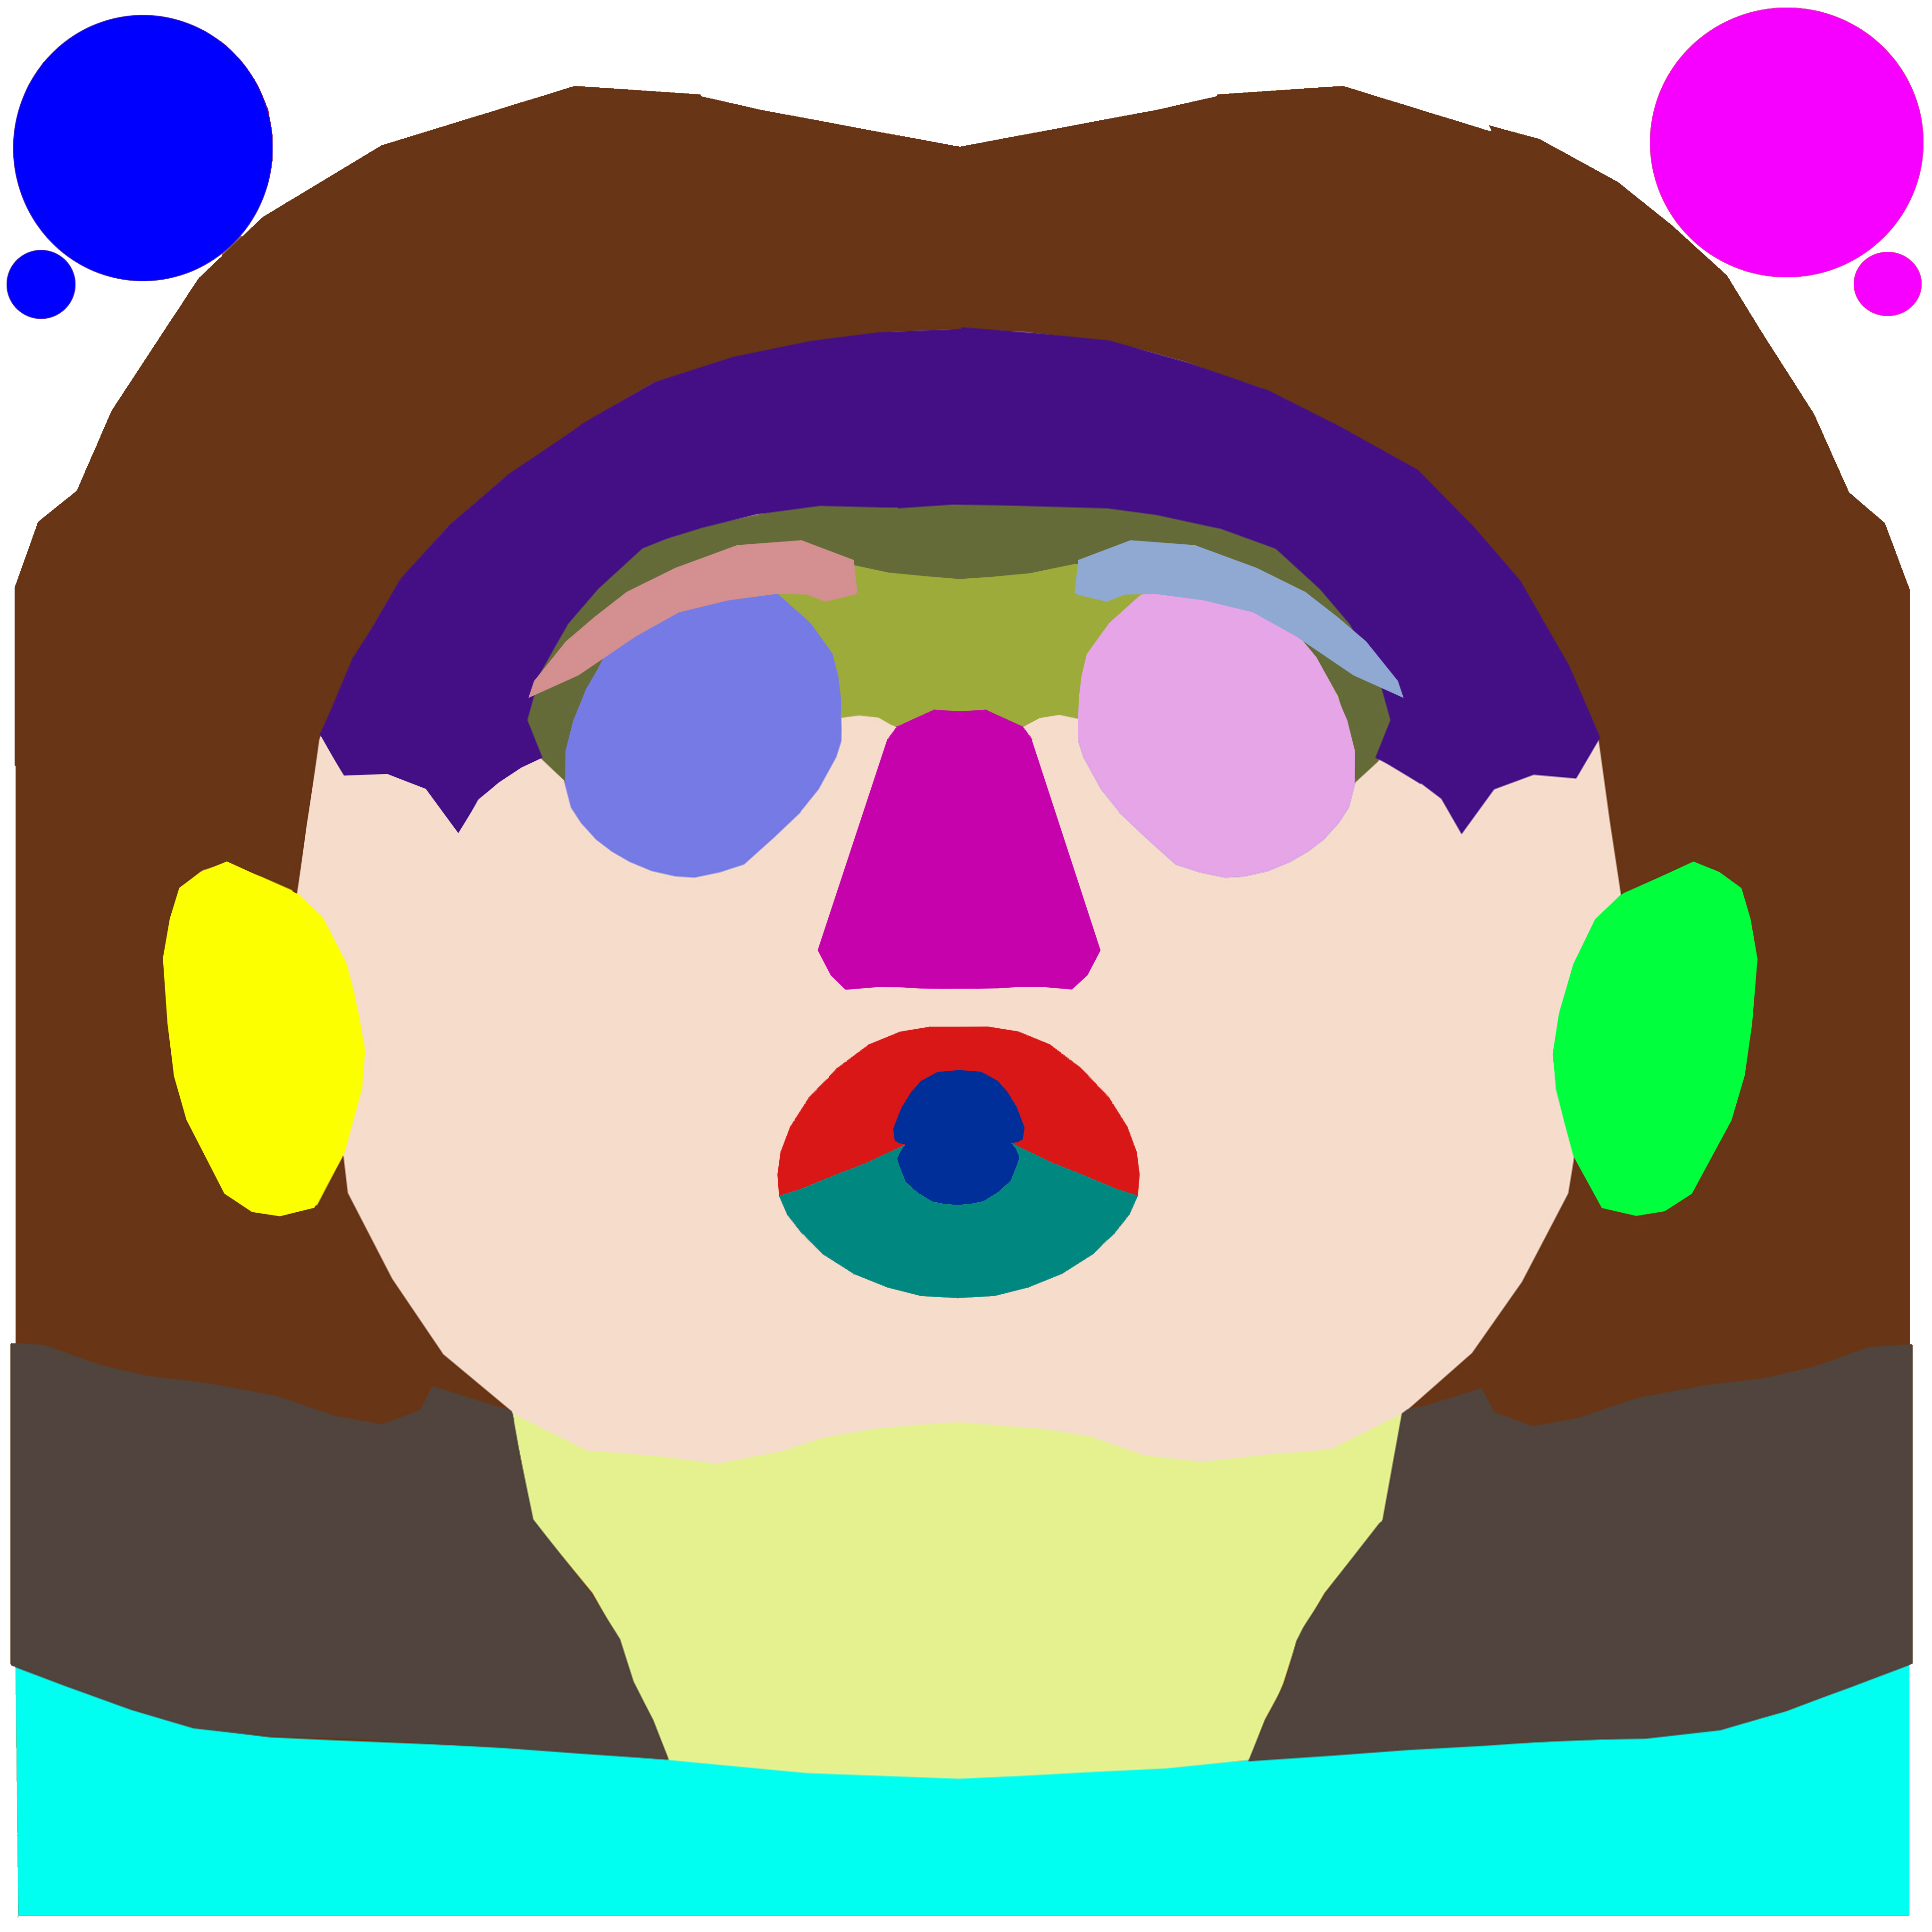}
        \caption{Flame texture}
        \label{fig:flame_uv}
    \end{subfigure}
    \begin{subfigure}{0.45\columnwidth}
        \includegraphics[width=\columnwidth]{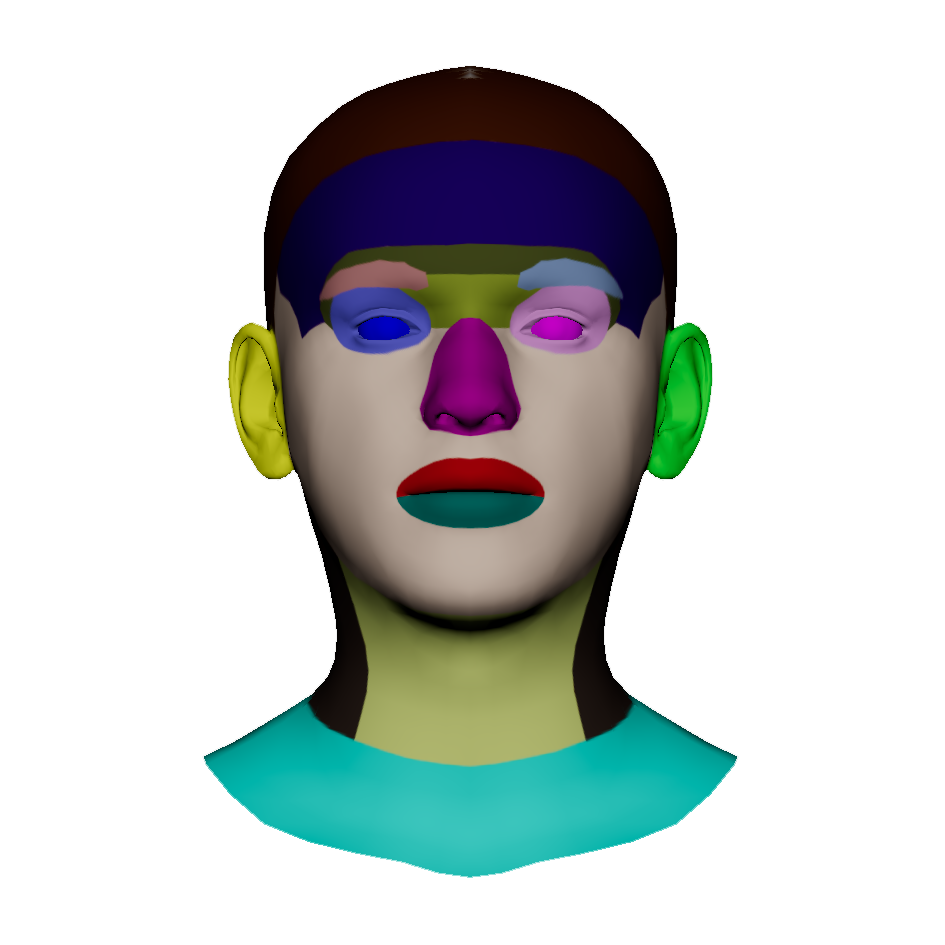}
        \caption{Flame texture on head}
        \label{fig:flame_tex}
    \end{subfigure}
    \caption{Flame head textured model with the semantic labels that are used for data and annotation generation.}
    \label{fig:flame_seg}
\end{figure}

\subsection{Next3D Processing}
Next3D introduces a sophisticated process for generating facial images, utilizing various modules to achieve high-fidelity and 3D-consistent avatars. Each module plays a critical role in the generation process:

\paragraph{Generative Texture-Rasterized Tri-Planes ($G_{texture}$, $T_{uv}$):} This module synthesizes neural textures through a StyleGAN2 CNN generator. The generated textures are rasterized to a screen-space feature map, based on a template mesh (e.g., the FLAME template), effectively combining explicit deformation control with the flexibility of implicit volumetric representation.

\paragraph{Mouth Synthesis Module ($G_{teeth}$):} Specifically designed to address the limitations of the FLAME template in representing the mouth interior, this module completes the mouth's interior features. It processes the extracted features and blends them into the feature planes, enhancing the realism and quality of the synthesized facial images.

\paragraph{Modeling Static Components ($G_{static}$):} For static parts of the face such as hair and background, Next3D employs a separate tri-plane branch generated by another StyleGAN2 CNN generator. This module ensures the consistent appearance of static facial components during animations and different expressions.

\paragraph{Neural Blending($T_{uv}'$):} This component takes the generated static features and the triplane features after mouth synthesis, and applies an alpha blending based on the frontal-face mask. Then applies a neural blending through a Conditional StyleGAN CNN to generate the final Triplane features.

\paragraph{Neural Rendering ($c, \sigma$):} This process involves projecting and sampling features from the tri-planes, and then decoding them into volume density and feature vectors. A super-resolution module interprets these into higher-resolution RGB images, crucial for the final image quality and resolution.

Each of these modules contributes to the overall effectiveness of the Next3D process in creating realistic and consistent facial avatars from unstructured 2D images. The synergy among them is key to the high-quality output of the generation process.

\subsection{Alignment Module}
The motivation for the alignment module lies in the lack of exact mapping which occurs in some cases due to the generative modules (StyleGAN2 blocks) in the data synthesis pipeline. Consequently, some affine adjustments to the 3D FLAME mesh are done so as to align better with the generated image and account for any camera projection inconsistencies in the final output.

\begin{figure}[h]
    \centering
    \includegraphics[width=\columnwidth]{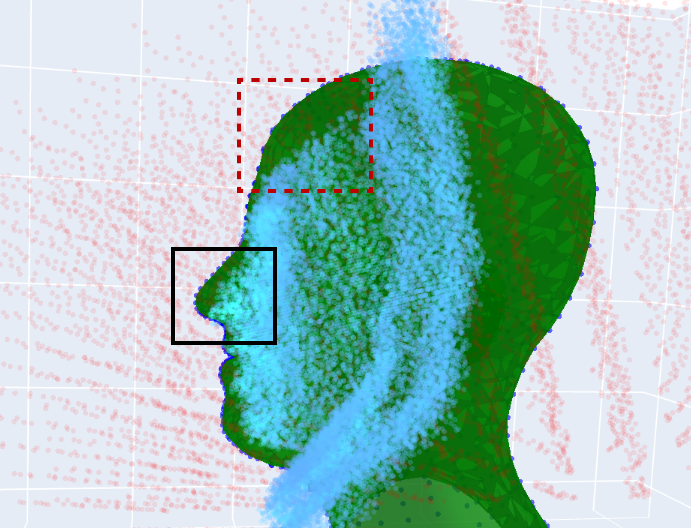}
    \caption{Visualization to highlight the need for alignment. The area in green shows the FLAME mesh in transformed camera co-ordinates, the points in light blue are taken from the level-set of the volumetric representation, and the red points are sampled along camera rays. The black box shows the alignment issue which can be fixed with affine transformaitons, and the red (dotted) box shows alignment issues arising due to the generative nature of the approach.}
    \label{fig:alignment}
\end{figure}

For a visual examination of the misalignment, we highlight fig \ref{fig:alignment}. In this image, we take the 3D FLAME mesh transformed to the camera 3D coordinates using the extrinsic matrix, and compare it's alignment with a level-set of the volumetric representation for a given sample, denoted by points $v_\alpha$. The level set is extracted along points on the sampled camera rays where the predicted volumetric density $\sigma(r(t_j))$ is compared against some threshold $\alpha$, such that $v_\alpha = \{r(t_j) | \sigma(r(t_j) \geq \alpha \}$, where $t_j$ denotes the point along the ray. The level set allows us to estimate approximate 3D representation of the head image in the generated space and compare it with the FLAME mesh which is used as the control input for the generation process. We observe two types of misalignments: Linear changes, which can be handled through a simple affine transformation on the 3D mesh; and, non-linear changes which arise due to the generative modules, specifically at the neural blending stage in the Next3D pipeline. The non-linear changes appear to be nominal and adding a non-linear adjustment without dense supervision will result in inconsistencies in the alignment process.

\begin{figure}[t]
  \includegraphics[width=0.98\columnwidth]{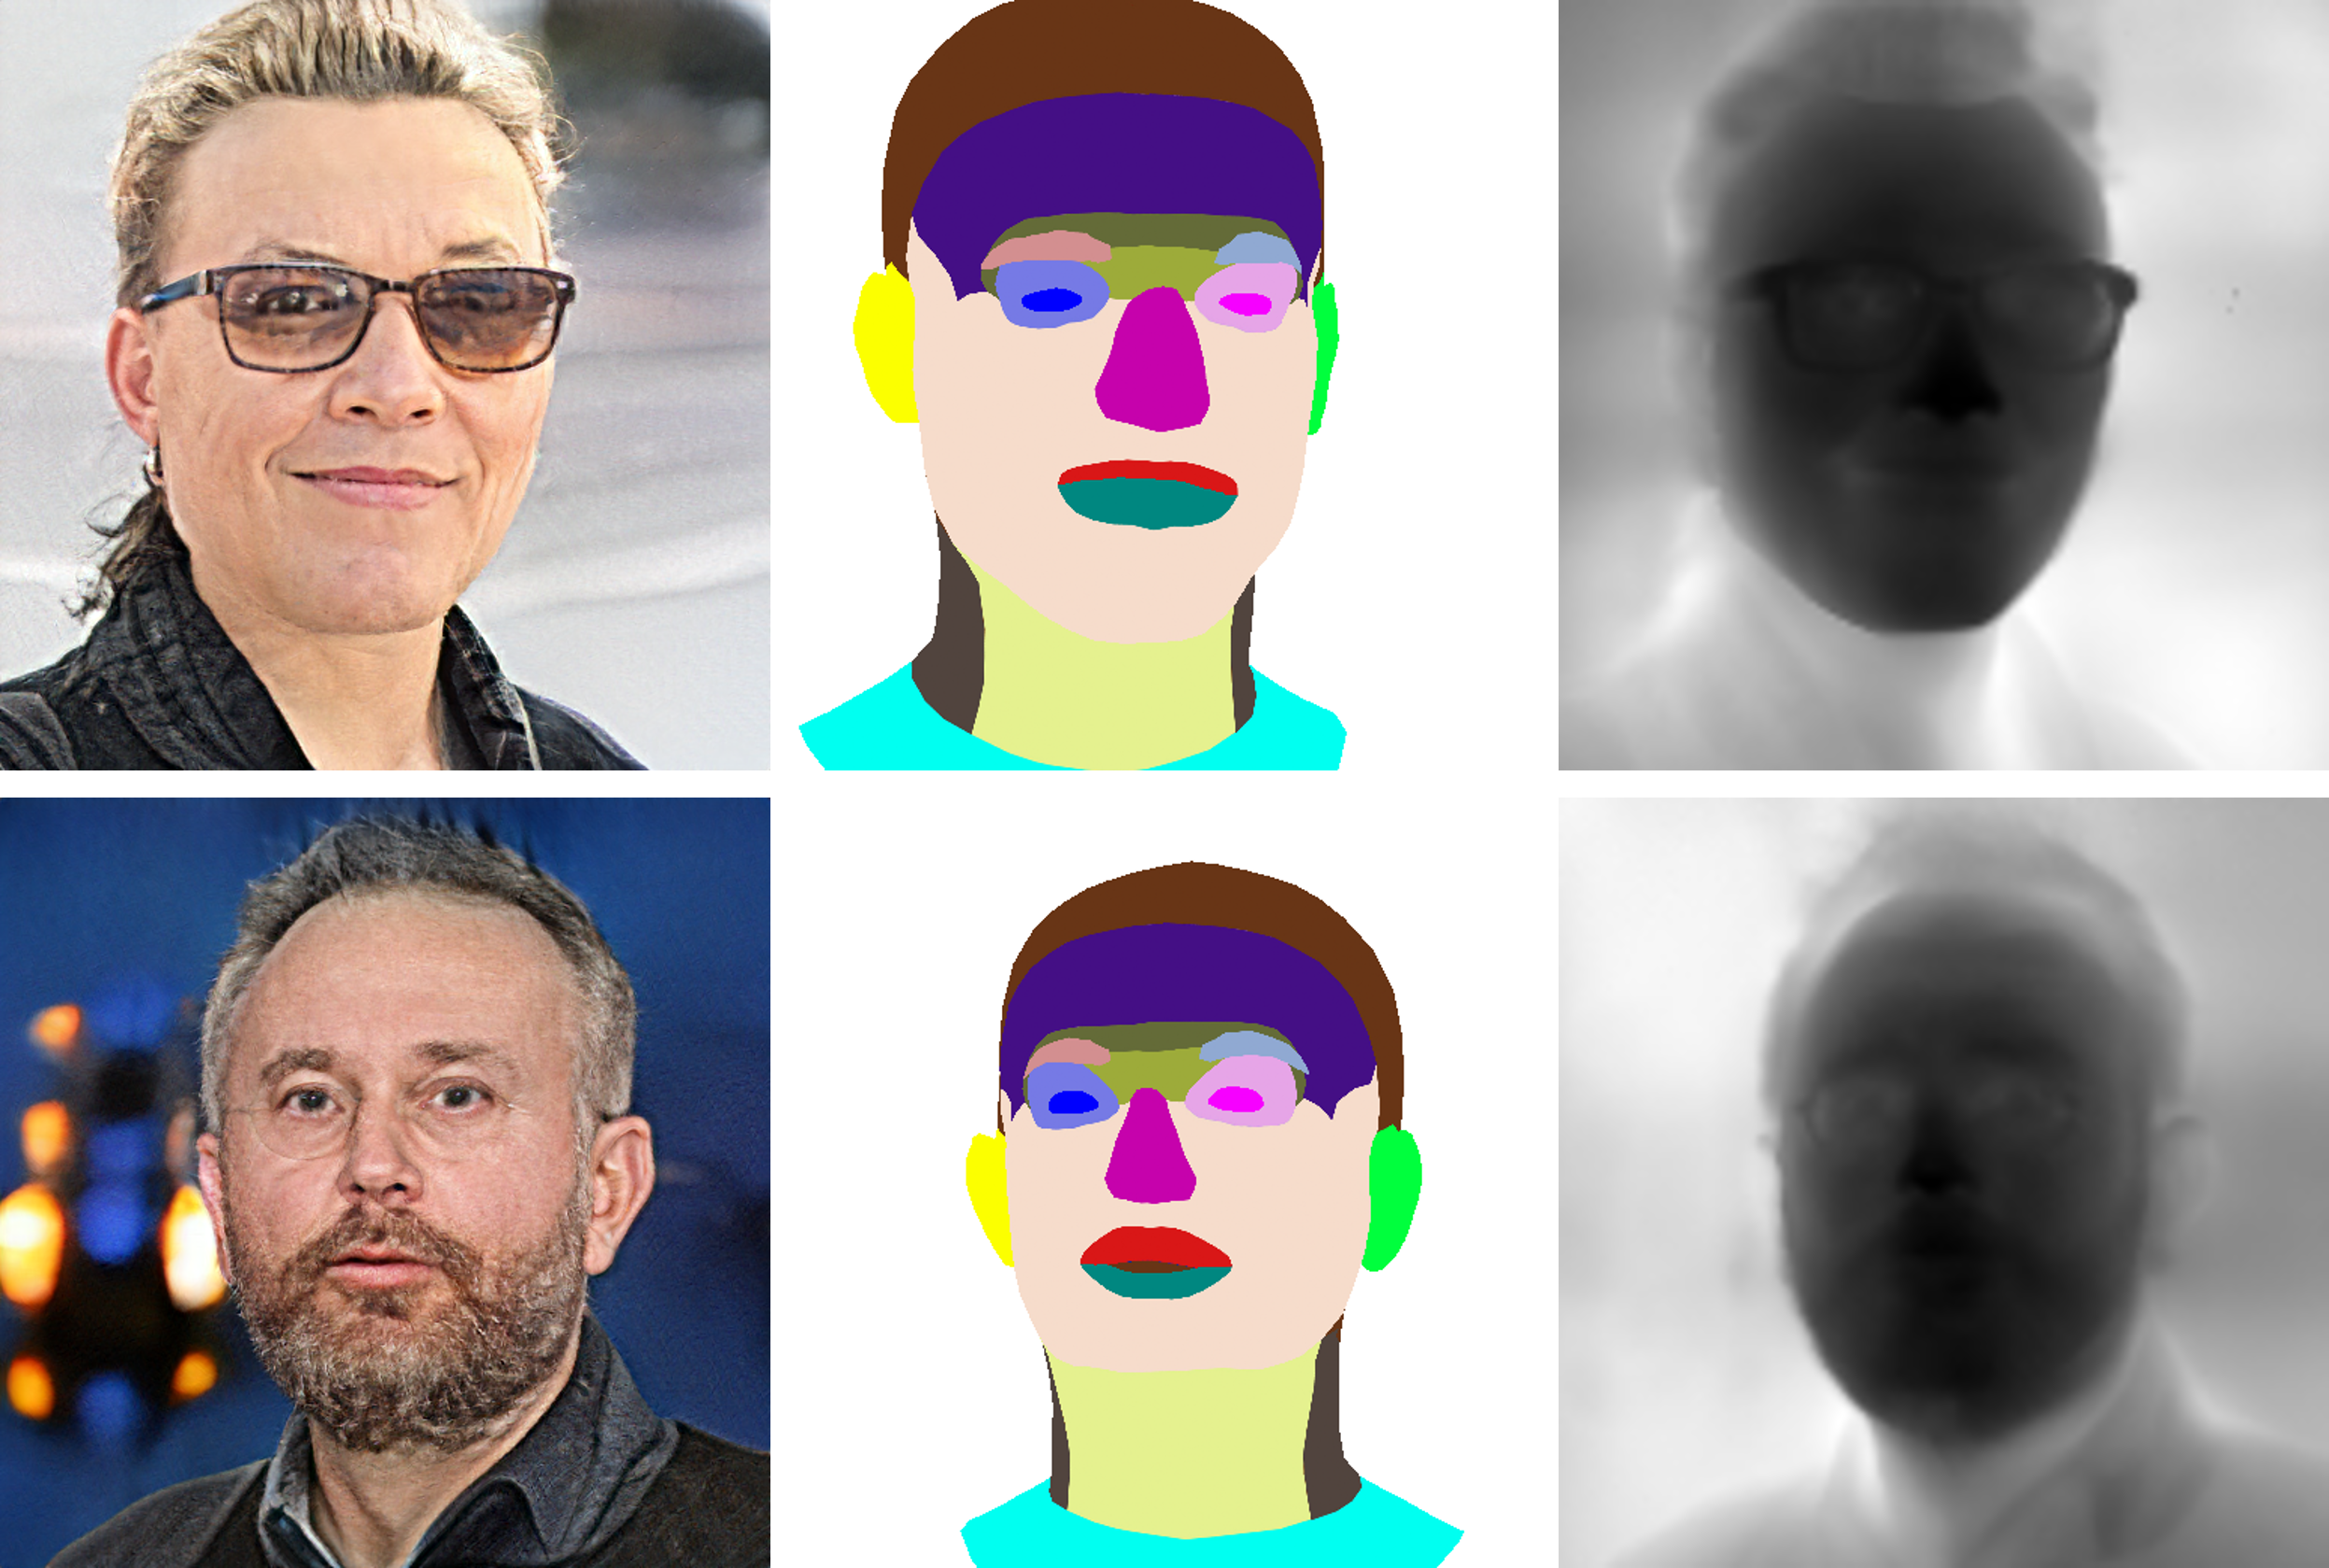}
  \caption{Generated data with segmentation and depth.}
  \label{fig:data}
\end{figure}

We use a affine transformation on the 3D FLAME mesh before transformation to the camera co-ordinate system, denoted by $(T_a)$, the alignment transformation is some arbitrary matrix applied on the initial FLAME vertices $v_a = T_a \cdot v$ and then rest of the camera transformation equations follow to obtain $v_c = [R | t] \cdot T_a \cdot v$. To optimize $T_a$, we consider a loss metric between the depth map generated in the Next3D pipeline and the depth generated from rendering the FLAME mesh frontal face using the transformed coordinates. Additionally, we can also compute the chamfer distance between the transformed landmarks $(l_c = [R | t] \cdot T_a \cdot l)$ and the level set points $v_\alpha$. The resulting error terms are as follows:

\begin{equation}
    \mathcal{L}_{\text{depth}} = \sum_{\text{pixels}} |D_{\text{Next3D}}(\text{pixel}) - D_{\text{FLAME}}(\text{pixel})|^2
\end{equation}

Where $D_{\text{Next3D}}$ and $D_{\text{FLAME}}$ are the depths from the synthetic pipeline and the depth map rendered through the Pytorch3D pipeline (along with semantic segmentation), respectively. The loss term $\mathcal{L}_{\text{depth}}$ is coupled with the chamfer loss as shown below:

\begin{equation}
    \mathcal{L}_{\text{chamfer}} = \sum_{l_i \in l_c} \min_{v_i \in v_\alpha} \| l_i - v_i \|^2 + \sum_{v_i \in v_\alpha} \min_{l_i \in l_c} \| v_i - l_i \|^2
\end{equation}

These loss functions guide the optimization of \( T_a \) to align the FLAME mesh with the generated image more accurately, thereby compensating for any inconsistencies introduced during the generative process.

\subsection{Annotation Generation}
Following the process in Next3D generative pipeline, we transform the 3D points from the FLAME mesh $v$ according to any geometric transformation that would affect the positions of the features. 

\paragraph{2D/3D Landmarks: }Apart from initial preprocessing for rasterization, the FLAME vertices are not directly changed in the Next3D pipeline, and hence using the projection matrix $P = K \cdot [R|t]$ on the FLAME vertices, we can get the projected landmarks on the 2D generated image.

\paragraph{Segmentation: } Similar to the landmark generation process, we re-create a camera object in Pytorch3D \cite{ravi2020pytorch3d} along with the corresponding textures of the FLAME mesh extracted from the UV mapping. Then the mesh is rendered with ambient lightning and non-specular surface to obtain the colored segmentation map of the projected mesh similar to  fig. \ref{fig:flame_seg}.

\paragraph{Depth: } We directly utilise the volume rendering pipeline, specifically the properties of NeRF \cite{nerf} to extract the depth based on the expected ray-length from the predicted densities $(\sigma)$ along each camera ray. In our setting, depth extraction from the Neural Radiance Fields (NeRF) pipeline employs a discrete approximation method for volume rendering. The depth \( D(\mathbf{r}) \) along a camera ray \( \mathbf{r} \), defined by its origin \( \mathbf{o} \) and direction \( \mathbf{d} \), is computed as a sum over sampled points along the ray. Specifically, for a set of sampled distances \( \{t_i\}_{i=1}^{N} \) along the ray \( \mathbf{r} \), where \( N \) is the number of samples, the depth is approximated as 

\begin{equation}
    D(\mathbf{r}) \approx \sum_{i=1}^{N} t_i \cdot \sigma(\mathbf{r}(t_i)) \cdot T_i \cdot \Delta t_i
\end{equation}

Where, \( \sigma(\mathbf{r}(t_i)) \) represents the predicted density at the point \( \mathbf{r}(t_i) = \mathbf{o} + t_i\mathbf{d} \), \( T_i \) is the accumulated transmittance up to distance \( t_i \), computed as:

\begin{equation}
T_i = \exp\left(-\sum_{j=1}^{i-1} \sigma(\mathbf{r}(t_j)) \cdot \Delta t_j\right)
\end{equation}

and \( \Delta t_i \) is the distance between adjacent samples. This approach provides a practical and efficient means to compute the expected depth along each camera ray based on the volumetric properties defined by NeRF.

We highlight the quality of the generated annotations in fig. \ref{fig:data}. However, note that when we consider the cases when the camera is not in a frontal pose to the face, the annotations can be misaligned to the actual generated image. On further investigation, we find that these inconsistencies arise due to the inherent behaviour of the generative models in the Next3D pipeline. 
% It is especially clear when we notice the feature mapping from Next3D for the given image in fig. \ref{}. Towards the correction of such discrepancies between the generated image and the annotation, we propose an alignment module.

\begin{figure}[t]
  \includegraphics[width=0.98\columnwidth]{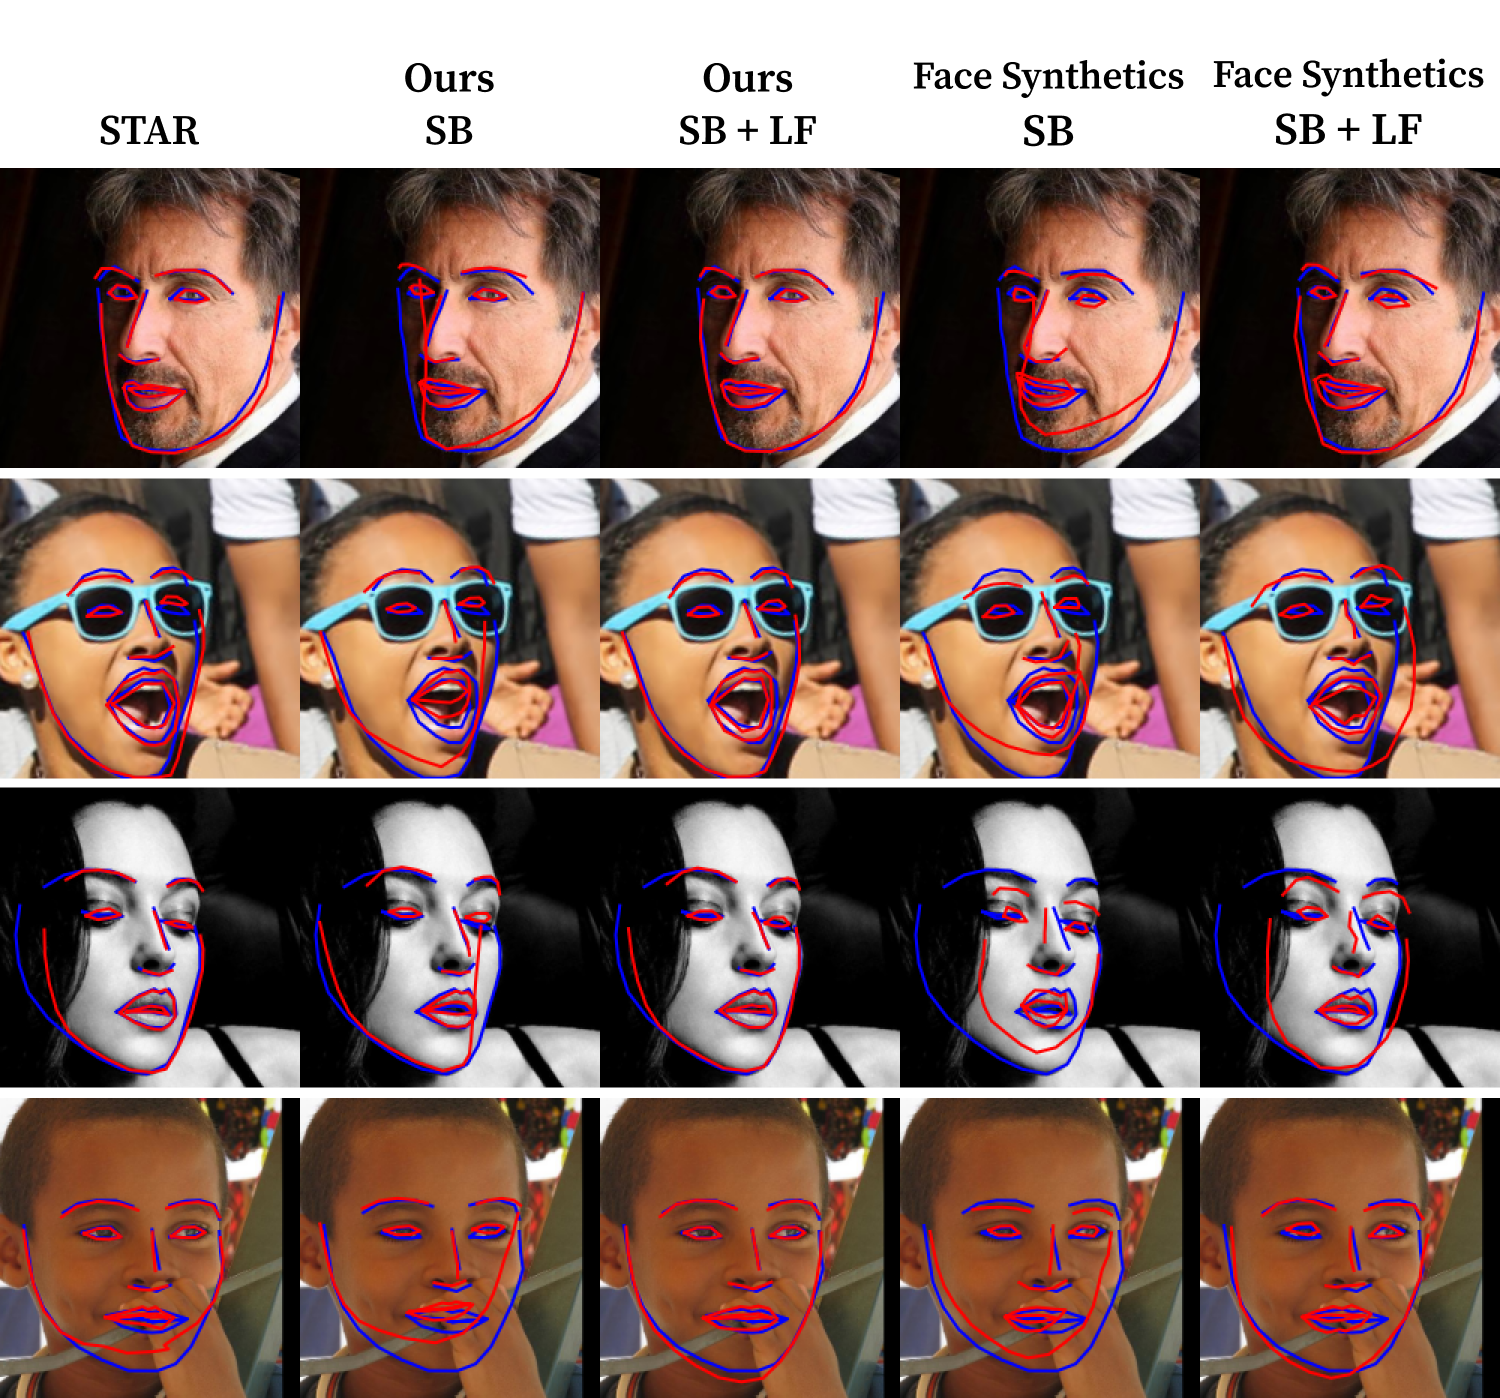}
  \caption{Landmark Localisation on 300W dataset. All models are trained on 300W. Gound truth is blue and model predictions are visualized in red.}
  \label{fig:300_300}
\end{figure}

\begin{figure}[t]
  \includegraphics[width=0.98\columnwidth]{sec/images/300w on Lapa.png}
  \caption{Landmark Localisation on LaPa dataset. All models are trained on 300W. Gound truth is blue and model predictions are visualized in red.}
  \label{fig:300_lapa}
\end{figure}

\section{Qualitative Results}
\label{sec:more_results}
In this section, we thoroughly compare our method with existing state of the art approaches in various settings.
For all the images that follow, we use SB to denote the output of our synthetic backbone and (SB + LF) for the outputs from the label finetuned model.

We compare our method with state-of-the-art models on different tasks and also with a recent synthetic data generated using physics based rendering \cite{fitymi} - Face Synthetics Dataset.
For comparing our method with \cite{fitymi}, we first train the multi-task backbone and then perform the label finetuning step to bridge the label discrepancy between the synthetic and real datasets.

We highlight that for all our experiments we use the same synthetic backbone (SB), which is then finetuned to compare against methods on a particular benchmark.
The qualitative results we show demonstrate the robustness of our synthetic backbone and its ability to generalize across any real world facial analysis dataset (keypoint, segmentation or depth). 

\subsection{Landmark Localisation}
We compare our method with state-of-the-art landmark localization model, STAR \cite{star} and a model trained using the Face Synthetics Dataset \cite{fitymi}.

In figure \ref{fig:300_300}, we can clearly see our method's superior performance against the state-of-the-art models on the 300w dataset.

We also show the robustness of our model in contrast to the existing approaches when evaluated on different datasets - LaPa and CelebA-Mask-HQ.
To this end, we show results for face alignment on LaPa and CelebA-Mask-HQ datasets using the models trained on 300W.

Figure \ref{fig:300_lapa} compares our model with the prior art when evaluated on the LaPa dataset.
For LaPa dataset we have 106 landmark annotations for the face as ground truth, which we show marked in blue.

We also show qualitative comparision on the CelebA-Mask-HQ dataset in figure \ref{fig:300_celeba}.
CelebA-Mask-HQ dataset contains only 5 landmark annotations, hence we only show each model's prediction in figure \ref{fig:300_celeba}  

\begin{figure}[t]
  \includegraphics[width=0.98\columnwidth]{sec/images/300w on CelebA.png}
  \caption{Landmark Localisation on CelebA-Mask dataset. All models are trained on 300W.}
  \label{fig:300_celeba}
\end{figure}

\begin{figure}[h!]
  \includegraphics[width=0.98\columnwidth]{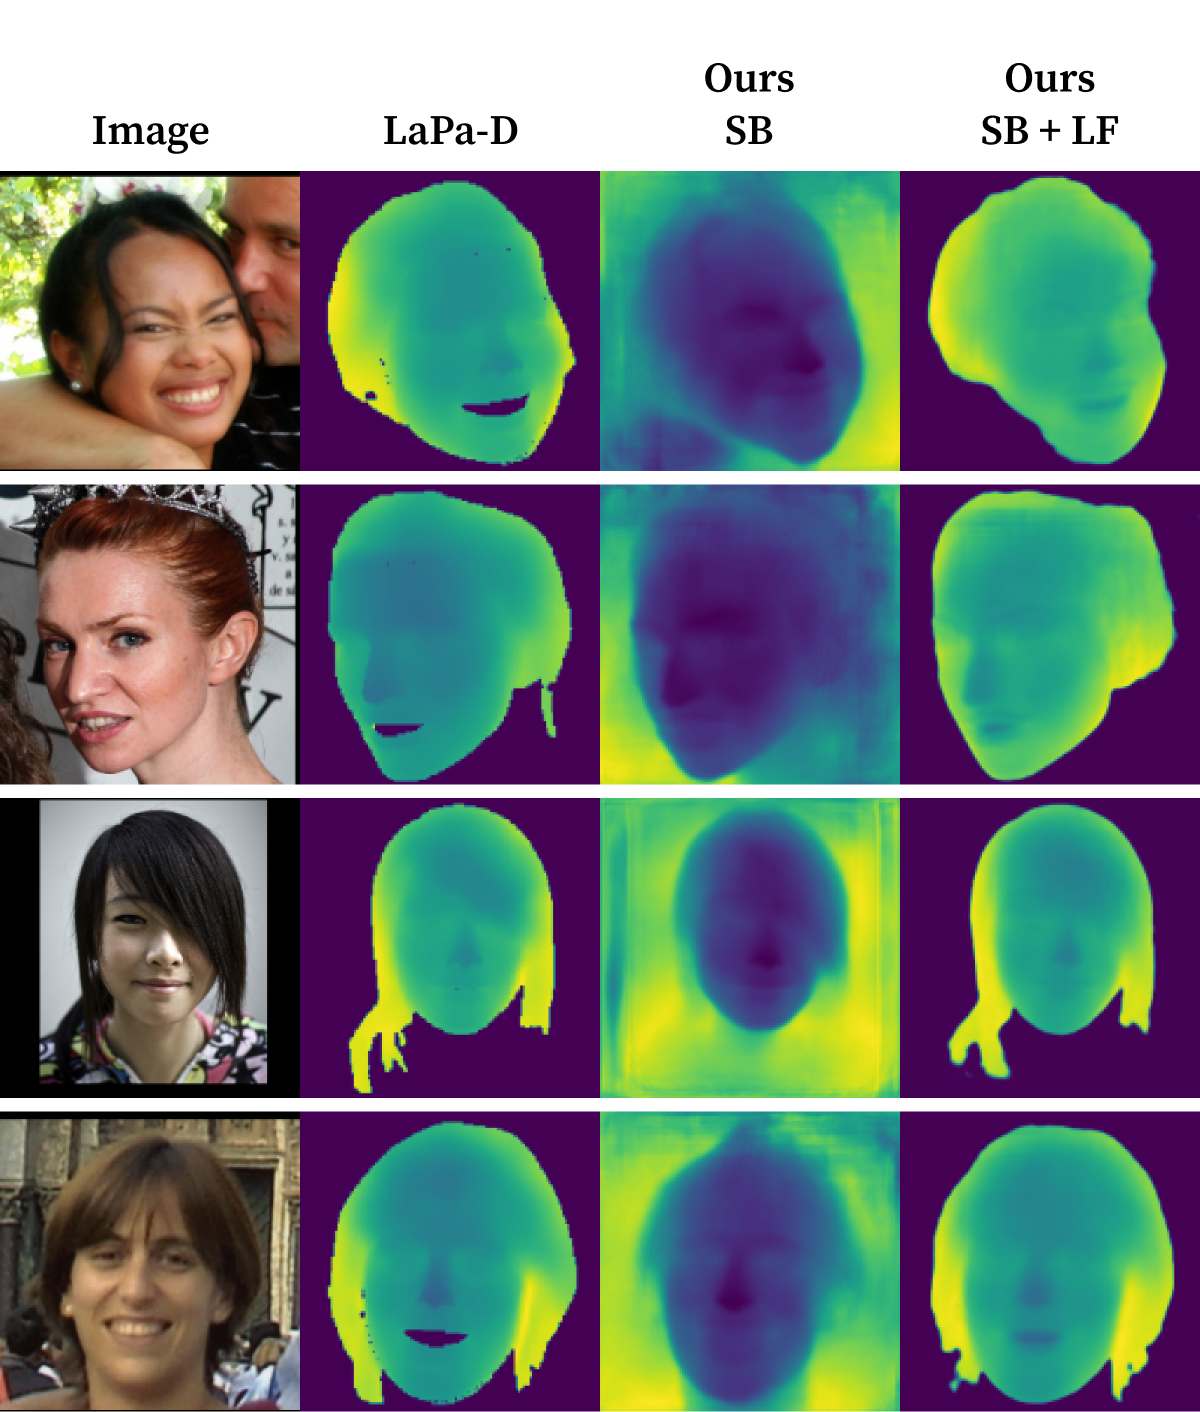}
  \caption{Depth predictions on LaPa-D dataset.}
  \label{fig:depth_lapa}
\end{figure}

\subsection{Depth}
In figure \ref{fig:depth_lapa} we show the qualitative results for depth.
We compare the results with the LaPa-D dataset.
Lapa-D is an extended version of LaPa with depth annotations fom an existing depth estimation model \cite{}. 
We observe that the depth predictions from our synthetic backbone is qualitatively superior.
This is because our synthetic backbone is trained on depth images rendered using volumetric rendering in our data generation step.
Label finetuning on LaPa-D is done to compare the results with the LaPa-D validation set.
% Rendering depth this way leads to better details a

\subsection{Face Parsing}
We show qualitative performance of our method on Face parsing task on both CelebA-Mask-HQ and LaPa datasets.
We compare our method with RTNet \cite{lin2021roi} and a model trained on the Face Synthetics dataset \cite{fitymi}.
For a fair comparison, the models trained with the Face Synthetics dataset are trained identically to our models.

Using the same synthetic backbone, we perform label finetuning for LaPa and CelebA-Mask-HQ and show our results across all datasets.

\paragraph{Finetuned with LaPa:} 
In figure \ref{fig:lapa_lapa}, we show results on samples from the LaPa test set.
We also evaluate on other datasets to compare the robustness of our method.
Figure \ref{fig:lapa_celeba} compares our method against the existing approaches on CelebA-Mask-HQ with model label-finetuned on LaPa Dataset.

We can clearly see that our synthetic backbone (SB) is able to predict the head segmentation mask quite accurately without label finetuning.
This shows that synthetic data alone is sufficient to train a robust facial analysis backbone.
The label finetuning process is to ensure a fair comparison with existing methods.

% LAPA
\begin{figure*}[t]
  \includegraphics[width=0.89\linewidth]{sec/images/Lapa on Lapa.png}
  \centering
  \caption{Face Parsing on LaPa dataset. Label Finetuning using LaPa dataset.}
  \label{fig:lapa_lapa}
\end{figure*}

\begin{figure*}[b]
  \includegraphics[width=0.89\linewidth]{sec/images/Lapa on CelebA.png}
  \centering
  \caption{Face Parsing on CelebA-Mask dataset. Label Finetuning using LaPa dataset.}
  \label{fig:lapa_celeba}
\end{figure*}

\paragraph{Finetuned with CelebA-Mask-HQ:}
In figure \ref{fig:celeba_celeba}, we show results on samples from the CelebA-Mask-HQ test set.
In addition to this, we also evaluate the performance of our model on the LaPa dataset.
When compared to other methods, in figure \ref{fig:celeba_lapa} we can clearly see that the performance of our model is on par with state of the art methods.

\section{Limitations}

We note that one of the primary limitation of our approach is the occasional misalignments observed between the generated faces and their corresponding annotations.
This stems from our choice of the generative model (Next3D) used for generating images.
Secondly, although we strive to generate data with high variance, certain cases like occlusions (both internal and external) and not generated using our current approach.

FLAME doesn't support hair, facial accessories and cloth, and therefore, our synthetic backbone is not trained on such classes.
We have to rely on label-finetuning for getting predictions for these classes.

% \begin{figure}[h]
%   \includegraphics[width=0.98\columnwidth]{sec/images/Lapa on 300w.png}
%   \caption{Face Parsing on 300W dataset. Label Finetuning using LaPa dataset.}
%   \label{fig:lapa_300}
% \end{figure}

% CELEBA
\begin{figure*}[t]
  \includegraphics[width=0.89\linewidth]{sec/images/CelebA on CelebA.png}
  \centering
  \caption{Face Parsing on CelebA-Mask dataset. Label Finetuning using CelebA-Mask dataset dataset.}
  \label{fig:celeba_celeba}
\end{figure*}

\begin{figure*}[b]
  \includegraphics[width=0.89\linewidth]{sec/images/CelebA on Lapa.png}
  \centering
  \caption{Face Parsing on LaPa dataset. Label Finetuning using CelebA-Mask-HQ dataset.}
  \label{fig:celeba_lapa}
\end{figure*}

% \begin{figure}[h]
%   \includegraphics[width=0.98\columnwidth]{sec/images/CelebA on 300w.png}
%   \caption{Face Parsing on 300W dataset. Label Finetuning using CelebA-Mask-HQ dataset.}
%   \label{fig:celeba_300}
% \end{figure}

% \begin{figure}[h]
%   \includegraphics[width=0.98\columnwidth]{sec/images/Lapa on Lapa.png}
%   \centering
%   \caption{Face Parsing on LaPa dataset. Label Finetuning using LaPa dataset.}
%   \label{fig:lapa_lapa}
% \end{figure}
% \pagebreak
